# Supplementary material for: A homogenized constrained mixture model of cardiac growth and remodeling: Analyzing mechanobiological stability and reversal
Source: arXiv:2203.12615 source file (2023-05-03)
Supplement: Supplementary file 2 [file metrics_i180.tex]

\def\myocytehomeostaticstressistagetwo{22.02277748047476}

\def\timepointbistagetwo{431.0}
\def\pressurebistagetwo{180.0}
\def\myocytestressbistagetwo{23.080600460769777}
\def\diameterbistagetwo{68.174556106555}
\def\wallthicknessbistagetwo{7.446502891513393}
\def\collagenmassfractionbistagetwo{0.2540101805038529}
