# Supplementary material for: A homogenized constrained mixture model of cardiac growth and remodeling: Analyzing mechanobiological stability and reversal
Source: arXiv:2203.12615 source file (2023-05-03)
Supplement: Supplementary file 3 [file metrics_r140.tex]

\def\midcavityrefwallthicknessrstageone{10.761044144526878}
\def\cavitydiameterrstageone{37.97108789828769}
\def\timepointarstageone{0.0}

\def\collagenmassfractionarstageone{0.1000022361719026}

\def\timepointbrstageone{1328.5}
\def\pressurebrstageone{140.0}
\def\myocytestressbrstageone{22.024182482227417}
\def\diameterbrstageone{45.487213640189964}
\def\wallthicknessbrstageone{9.501734110846582}
\def\collagenmassfractionbrstageone{0.12326161508607952}

\def\timepointcrstageone{1988.5}
\def\pressurecrstageone{120.0}
\def\myocytestresscrstageone{22.02170744001227}
\def\diametercrstageone{37.355680653048026}
\def\wallthicknesscrstageone{10.976109457287103}
\def\collagenmassfractioncrstageone{0.1028483246693137}
