# Supplementary material for: A homogenized constrained mixture model of cardiac growth and remodeling: Analyzing mechanobiological stability and reversal
Source: arXiv:2203.12615 source file (2023-05-03)
Supplement: Supplementary file 4 [file metrics_r180.tex]

\def\timepointbrstagetwo{151.0}

\def\timepointcrstagetwo{855.5}
\def\pressurecrstagetwo{120.0}
\def\myocytestresscrstagetwo{22.021674414018996}
\def\diametercrstagetwo{34.746034631548746}
\def\wallthicknesscrstagetwo{11.842800468885063}
\def\collagenmassfractioncrstagetwo{0.11438786875882459}
