# Supplementary material for: A homogenized constrained mixture model of cardiac growth and remodeling: Analyzing mechanobiological stability and reversal
Source: arXiv:2203.12615 source file (2023-05-03)
Supplement: Supplementary file 5 [file metrics_s140_0.33.tex]

\def\myocytehomeostaticstresspstagetwoa{22.02277748047476}
\def\midcavityrefwallthicknesspstagetwoa{10.761044144526878}
\def\cavitydiameterpstagetwoa{37.97807748655915}
\def\timepointapstagetwoa{0.0}
\def\pressureapstagetwoa{120.0}
\def\myocytestressapstagetwoa{22.021899769774404}
\def\diameterapstagetwoa{38.003314116920116}
\def\wallthicknessapstagetwoa{10.76100316923541}
\def\collagenmassfractionapstagetwoa{0.099990853076329}
\def\timepointbpstagetwoa{900.5}
\def\pressurebpstagetwoa{140.0}
\def\myocytestressbpstagetwoa{22.320175704857355}
\def\diameterbpstagetwoa{57.81977156698272}
\def\wallthicknessbpstagetwoa{8.326654638067867}
\def\collagenmassfractionbpstagetwoa{0.16063522753367787}
