# Supplementary material for: A homogenized constrained mixture model of cardiac growth and remodeling: Analyzing mechanobiological stability and reversal
Source: arXiv:2203.12615 source file (2023-05-03)
Supplement: Supplementary file 6 [file metrics_s140_1.tex]

\def\myocytehomeostaticstresspstagetwob{22.02277748047476}
\def\midcavityrefwallthicknesspstagetwob{10.761044144526878}
\def\cavitydiameterpstagetwob{37.99325395114782}
\def\timepointapstagetwob{0.0}
\def\pressureapstagetwob{120.0}
\def\myocytestressapstagetwob{22.02257643915123}
\def\diameterapstagetwob{37.990492240318716}
\def\wallthicknessapstagetwob{10.760539770234908}
\def\collagenmassfractionapstagetwob{0.1000022361719026}
\def\timepointbpstagetwob{1328.5}
\def\pressurebpstagetwob{140.0}
\def\myocytestressbpstagetwob{22.024182482227417}
\def\diameterbpstagetwob{45.47676555981399}
\def\wallthicknessbpstagetwob{9.501734110846582}
\def\collagenmassfractionbpstagetwob{0.12326161508607952}
