# Supplementary material for: A homogenized constrained mixture model of cardiac growth and remodeling: Analyzing mechanobiological stability and reversal
Source: arXiv:2203.12615 source file (2023-05-03)
Supplement: Supplementary file 7 [file metrics_s140_243.tex]

\def\myocytehomeostaticstresspstagetwog{22.02277748047476}
\def\midcavityrefwallthicknesspstagetwog{10.761044144526878}
\def\cavitydiameterpstagetwog{37.97111782504683}
\def\timepointapstagetwog{0.0}
\def\pressureapstagetwog{120.0}
\def\myocytestressapstagetwog{22.02278315597887}
\def\diameterapstagetwog{37.97098472426861}
\def\wallthicknessapstagetwog{10.761048550539796}
\def\collagenmassfractionapstagetwog{0.10000354766853382}
\def\timepointbpstagetwog{229.0}
\def\pressurebpstagetwog{140.0}
\def\myocytestressbpstagetwog{22.022761704238413}
\def\diameterbpstagetwog{38.4309170788811}
\def\wallthicknessbpstagetwog{10.562026691903824}
\def\collagenmassfractionbpstagetwog{0.10065572067861417}
