# Supplementary material for: A homogenized constrained mixture model of cardiac growth and remodeling: Analyzing mechanobiological stability and reversal
Source: arXiv:2203.12615 source file (2023-05-03)
Supplement: Supplementary file 9 [file metrics_s140_3.tex]

\def\myocytehomeostaticstresspstagetwoc{22.02277748047476}
\def\midcavityrefwallthicknesspstagetwoc{10.761044144526878}
\def\cavitydiameterpstagetwoc{37.973852415698175}
\def\timepointapstagetwoc{0.0}
\def\pressureapstagetwoc{120.0}
\def\myocytestressapstagetwoc{22.022758872012716}
\def\diameterapstagetwoc{37.988453536134145}
\def\wallthicknessapstagetwoc{10.760344155571936}
\def\collagenmassfractionapstagetwoc{0.10000947010343447}
\def\timepointbpstagetwoc{677.5}
\def\pressurebpstagetwoc{140.0}
\def\myocytestressbpstagetwoc{22.023592759552812}
\def\diameterbpstagetwoc{41.952050164040166}
\def\wallthicknessbpstagetwoc{9.98097168828223}
\def\collagenmassfractionbpstagetwoc{0.1120256682317859}
