# Supplementary material for: A homogenized constrained mixture model of cardiac growth and remodeling: Analyzing mechanobiological stability and reversal
Source: arXiv:2203.12615 source file (2023-05-03)
Supplement: Supplementary file 11 [file metrics_s140_9.tex]

\def\myocytehomeostaticstresspstagetwod{22.02277748047476}
\def\midcavityrefwallthicknesspstagetwod{10.761044144526878}
\def\cavitydiameterpstagetwod{37.97771347274108}
\def\timepointapstagetwod{0.0}
\def\pressureapstagetwod{120.0}
\def\myocytestressapstagetwod{22.022716368868238}
\def\diameterapstagetwod{37.975187375950405}
\def\wallthicknessapstagetwod{10.760440284747107}
\def\collagenmassfractionapstagetwod{0.10001182107091391}
\def\timepointbpstagetwod{424.5}
\def\pressurebpstagetwod{140.0}
\def\myocytestressbpstagetwod{22.023119725211615}
\def\diameterbpstagetwod{40.1632035746836}
\def\wallthicknessbpstagetwod{10.267605623789398}
\def\collagenmassfractionbpstagetwod{0.1060979560883707}
