# Supplementary material for: A homogenized constrained mixture model of cardiac growth and remodeling: Analyzing mechanobiological stability and reversal
Source: arXiv:2203.12615 source file (2023-05-03)
Supplement: Supplementary file 12 [file metrics_s180_0.33.tex]

\def\myocytehomeostaticstresspstagetwoa{22.02277748047476}
\def\midcavityrefwallthicknesspstagetwoa{10.761044144526878}
\def\cavitydiameterpstagetwoa{37.97807748655915}
\def\timepointapstagetwoa{0.0}
\def\pressureapstagetwoa{120.0}
\def\myocytestressapstagetwoa{22.021899769774404}
\def\diameterapstagetwoa{38.003314116920116}
\def\wallthicknessapstagetwoa{10.76100316923541}
\def\collagenmassfractionapstagetwoa{0.099990853076329}
\def\timepointbpstagetwoa{50.0}
\def\pressurebpstagetwoa{180.0}
\def\myocytestressbpstagetwoa{23.802518022443518}
\def\diameterbpstagetwoa{44.450459628454624}
\def\wallthicknessbpstagetwoa{9.803945208699716}
\def\collagenmassfractionbpstagetwoa{0.1206160142349238}
