# Supplementary material for: A homogenized constrained mixture model of cardiac growth and remodeling: Analyzing mechanobiological stability and reversal
Source: arXiv:2203.12615 source file (2023-05-03)
Supplement: Supplementary file 13 [file metrics_s180_1.tex]

\def\myocytehomeostaticstresspstagetwob{22.02277748047476}
\def\midcavityrefwallthicknesspstagetwob{10.761044144526878}
\def\cavitydiameterpstagetwob{37.99325395114782}
\def\timepointapstagetwob{0.0}
\def\pressureapstagetwob{120.0}
\def\myocytestressapstagetwob{22.02257643915123}
\def\diameterapstagetwob{37.990492240318716}
\def\wallthicknessapstagetwob{10.760539770234908}
\def\collagenmassfractionapstagetwob{0.1000022361719026}
\def\timepointbpstagetwob{431.0}
\def\pressurebpstagetwob{180.0}
\def\myocytestressbpstagetwob{23.080600460769777}
\def\diameterbpstagetwob{68.19942571701}
\def\wallthicknessbpstagetwob{7.446502891513393}
\def\collagenmassfractionbpstagetwob{0.2540101805038529}
