# Supplementary material for: A homogenized constrained mixture model of cardiac growth and remodeling: Analyzing mechanobiological stability and reversal
Source: arXiv:2203.12615 source file (2023-05-03)
Supplement: Supplementary file 15 [file metrics_s180_27.tex]

\def\myocytehomeostaticstresspstagetwoe{22.02277748047476}
\def\midcavityrefwallthicknesspstagetwoe{10.761044144526878}
\def\cavitydiameterpstagetwoe{37.98754296280138}
\def\timepointapstagetwoe{0.0}
\def\pressureapstagetwoe{120.0}
\def\myocytestressapstagetwoe{22.022684177941386}
\def\diameterapstagetwoe{37.975881882052676}
\def\wallthicknessapstagetwoe{10.76075600740356}
\def\collagenmassfractionapstagetwoe{0.10000796488464152}
\def\timepointbpstagetwoe{406.5}
\def\pressurebpstagetwoe{180.0}
\def\myocytestressbpstagetwoe{22.02293782974717}
\def\diameterbpstagetwoe{41.602204405454316}
\def\wallthicknessbpstagetwoe{9.843481427441295}
\def\collagenmassfractionbpstagetwoe{0.11028213619192251}
