# Supplementary material for: A homogenized constrained mixture model of cardiac growth and remodeling: Analyzing mechanobiological stability and reversal
Source: arXiv:2203.12615 source file (2023-05-03)
Supplement: Supplementary file 17 [file metrics_s180_81.tex]

\def\myocytehomeostaticstresspstagetwof{22.02277748047476}
\def\midcavityrefwallthicknesspstagetwof{10.761044144526878}
\def\cavitydiameterpstagetwof{37.973171234540985}
\def\timepointapstagetwof{0.0}
\def\pressureapstagetwof{120.0}
\def\myocytestressapstagetwof{22.0227338109269}
\def\diameterapstagetwof{37.9659369685692}
\def\wallthicknessapstagetwof{10.760952666167386}
\def\collagenmassfractionapstagetwof{0.1000049472779319}
\def\timepointbpstagetwof{331.0}
\def\pressurebpstagetwof{180.0}
\def\myocytestressbpstagetwof{22.022886994010456}
\def\diameterbpstagetwof{39.99044759552984}
\def\wallthicknessbpstagetwof{10.085092917227717}
\def\collagenmassfractionbpstagetwof{0.10421860464531123}
