# Supplementary material for: A homogenized constrained mixture model of cardiac growth and remodeling: Analyzing mechanobiological stability and reversal
Source: arXiv:2203.12615 source file (2023-05-03)
Supplement: Supplementary file 18 [file metrics_s180_9.tex]

\def\myocytehomeostaticstresspstagetwod{22.02277748047476}
\def\midcavityrefwallthicknesspstagetwod{10.761044144526878}
\def\cavitydiameterpstagetwod{37.97771347274108}
\def\timepointapstagetwod{0.0}
\def\pressureapstagetwod{120.0}
\def\myocytestressapstagetwod{22.022716368868238}
\def\diameterapstagetwod{37.975187375950405}
\def\wallthicknessapstagetwod{10.760440284747107}
\def\collagenmassfractionapstagetwod{0.10001182107091391}
\def\timepointbpstagetwod{756.0}
\def\pressurebpstagetwod{180.0}
\def\myocytestressbpstagetwod{22.02326579967937}
\def\diameterbpstagetwod{45.99104445918943}
\def\wallthicknessbpstagetwod{9.220541197362996}
\def\collagenmassfractionbpstagetwod{0.12785873909585707}
